# Supplementary material for: Renormalization of parton quasi-distributions beyond the leading order: spacelike vs. timelike
Source: arXiv:2004.01043 ancillary file (2020-04-02)
Supplement: Supplementary file 1 [file README.pdf]

Files `correlators.mres`, `ad.mres` and `rc.mres` contain the MATHEMATICA versions (in general covariant gauge and for general gauge group) of the expressions given in Sections 6 and Appendixes A and B of the paper

V. M. Braun, K. G. Chetyrkin and B. Kniehl “Three-loop renormalization of parton quasi-distributions: spacelike vs. timelike”.

### Notations:

`xil = 1 - xi`, `xi = ξ`: gauge parameter (`xil=0` -> Landau gauge, `xil=1` -> Feynman gauge); the tree gluon propagator reads:

$$D_{\alpha\beta}(q) = \frac{-g_{\alpha\beta}}{-q^2} + \xi \frac{q_\alpha q_\beta}{q^4}.$$

`z3`, `z5` stand for the values of the Riemann zeta-function with `z3 = ζ3 = 1.2020569...`, `z5 = ζ5 = 1.0369278...`

`cf = CF` and `ca = CA` are the quadratic Casimir operators of the quark  $[T^a T^a]_{ij} = C_F \delta_{ij}$  and the adjoint  $[C^a C^a]_{bd} = C_A \delta_{bd}$ ,  $(C^a)_{bc} = -if^{abc}$  representations of the Lie algebra, `ng` and `dr` are dimensions of the adjoint (gluon) and quark representations of the gauge group, `nf` stands for the number of quark flavors and `tr = Tf` refers to the trace normalization  $\text{tr}(T^a T^b) = T_f \delta^{ab}$ .

Finally, `om = ω = pv`, `vv = v · v` and

$$\text{tLn} = \ln \frac{\mu}{-2\omega}, \text{sLn} = \ln \frac{\mu}{2\omega}, \text{xLn} = \ln \left( \frac{\mu i t e^{\gamma_E}}{2} \right), \text{zLn} = \ln \left( \frac{\mu z e^{\gamma_E}}{2} \right),$$

with  $\gamma_E = 0.577216\dots$ , being the Euler constant appearing in the expansion of the Gamma function

$$\Gamma(1 + \epsilon) = 1 - \gamma_E \epsilon + \mathcal{O}(\epsilon^2).$$

File `correlators.mres` contains expressions

`tSigma`, `sSigma`, `tD`, `sD`, `tDtt`, `sDtt`, `tDpt`, `sDpt`, `zPitt`, `xPitt`, `zPipt`, `xPipt`

which correspond to the functions

$$\Sigma(v^2 = 1), \Sigma(v^2 = -1), tD(v^2 = 1), \tilde{D}(v^2 = -1), \tilde{D}_{\perp\perp}(v^2 = 1), \tilde{D}_{\perp\perp}(v^2 = -1), \tilde{D}_{\parallel\perp}(v^2 = 1), \tilde{D}_{\parallel\perp}(v^2 = -1), \Pi_{\perp\perp}(z, v^2 = -1), \Pi_{\perp\perp}(t, v^2 = 1), \Pi_{\parallel\perp}(z, v^2 = -1), \Pi_{\parallel\perp}(t, v^2 = 1).$$

Note, that have used a symbol `Im1`  $\equiv i \equiv \sqrt{-1}$  instead of the Mathematica symbol `I` for the the imaginary unit. A symbol `x` is introduced as convenient label in the relation (see eq. (3.43) of the main text of the paper)

$$\text{tLn} \rightarrow \text{sLn} + \text{x} * (\text{Im1} * \text{Pi}/2). \quad (1)$$

Within a Mathematica session it can always removed by saying

$$\text{x} = 1;$$

File `rc.mres` contains the renormalization constants `Za`, `Z2`, `Z3`, `ZQ`, `Z2h`, `Zpt`, `Ztt` (see Sections 3.1 and 3.2 of the paper).

File `ad.mres` contains the QCD  $\beta$ -function=`be`, as well as the corresponding ADs

$$\text{g2}=\gamma_2, \text{g3}=\gamma_3, \text{gQ}=\gamma_Q, \text{g2h}=\gamma_h, \text{gtt}=\gamma_{\perp\perp}, \text{gpt}=\gamma_{\parallel\perp}.$$

## Bibliography notes:

Many results given in the paper and in the auxiliary files were originally obtained by other authors and have been included by us for completeness. Below we cite the corresponding works. Note that all results for ADs  $\gamma_h, \gamma_Q$  and for the VEV  $\Pi$  cited below correspond to the timelike choice of the vector  $v$  with  $v \cdot v = 1$ .

The anomalous dimension (AD)  $\gamma_Q$  was computed at 1- 2- and 3-loops in [1, 2], [3, 4] and [5] respectively.

The anomalous dimension of the special “heavy” field  $h_v$  was first computed at 2- and 3-loop in [4] and [6] and confirmed later in [5] and even extended to 4 loops in [7, 8].

The VEV  $\Pi$  was computed at 2 loops in [4] and at 3 loops in [9].

The VEV of gluon off-light-cone operator  $\mathbb{G}_{\mu\nu\alpha\beta}$  in two loops was found in [10] and the corresponding 1-loop ADs first computed in [11, 12].

The 3-loop renormalization factors  $Z_3$ ,  $Z_2$  and  $Z_a$  are well-known since long [13, 14, 15].

## References

- [1] H. D. Politzer and M. B. Wise, *Leading Logarithms of Heavy Quark Masses in Processes with Light and Heavy Quarks*, *Phys. Lett.* **B206** (1988) 681–684.
- [2] M. A. Shifman and M. B. Voloshin, *On Annihilation of Mesons Built from Heavy and Light Quark and anti- $B^0 \longleftrightarrow B^0$  Oscillations*, *Sov. J. Nucl. Phys.* **45** (1987) 292.
- [3] X.-D. Ji and M. J. Musolf, *Subleading logarithmic mass dependence in heavy meson form-factors*, *Phys. Lett.* **B257** (1991) 409–413.
- [4] D. J. Broadhurst and A. G. Grozin, *Two loop renormalization of the effective field theory of a static quark*, *Phys. Lett.* **B267** (1991) 105–110, [[hep-ph/9908362](#)].
- [5] K. G. Chetyrkin and A. G. Grozin, *Three loop anomalous dimension of the heavy light quark current in HQET*, *Nucl. Phys.* **B666** (2003) 289–302, [[hep-ph/0303113](#)].
- [6] K. Melnikov and T. van Ritbergen, *The Three loop on-shell renormalization of QCD and QED*, *Nucl. Phys.* **B591** (2000) 515–546, [[hep-ph/0005131](#)].
- [7] P. Marquard, A. V. Smirnov, V. A. Smirnov and M. Steinhauser, *Four-loop wave function renormalization in QCD and QED*, *Phys. Rev.* **D97** (2018) 054032, [[1801.08292](#)].
- [8] R. Br user, A. Grozin, J. M. Henn and M. Stahlhofen, *Matter dependence of the four-loop QCD cusp anomalous dimension: from small angles to all angles*, *JHEP* **05** (2019) 186, [[1902.05076](#)].
- [9] A. Czarnecki and K. Melnikov, *Threshold expansion for heavy light systems and flavor off diagonal current current correlators*, *Phys. Rev.* **D66** (2002) 011502(R), [[hep-ph/0110028](#)].
- [10] M. Eidemuller and M. Jamin, *QCD field strength correlator at the next-to-leading order*, *Phys. Lett.* **B416** (1998) 415–420, [[hep-ph/9709419](#)].

- [11] H. Dorn and E. Wieczorek, *Renormalization and Short Distance Properties of String Type Equations in QCD*, *Z. Phys.* **C9** (1981) 49.
- [12] H. Dorn, D. Robaschik and E. Wieczorek, *Renormalization and short distance properties of gauge invariant gluonium and hadron operators*, *Annalen Phys.* **40** (1983) 166.
- [13] O. V. Tarasov, A. A. Vladimirov and A. Y. Zharkov, *The Gell-Mann-Low function of QCD in the three loop approximation*, *Phys. Lett.* **B93** (1980) 429–432.
- [14] O. V. Tarasov, *Anomalous dimensions of quark masses in the three-loop approximation*, 1910.12231.
- [15] S. A. Larin and J. A. M. Vermaseren, *The Three loop QCD Beta function and anomalous dimensions*, *Phys. Lett.* **B303** (1993) 334–336, [[hep-ph/9302208](#)].
